# Supplementary material for: Compacting Squares: Input-Sensitive In-Place Reconfiguration of Sliding Squares
Source: arXiv:2105.07997 source file (2021-12-14)

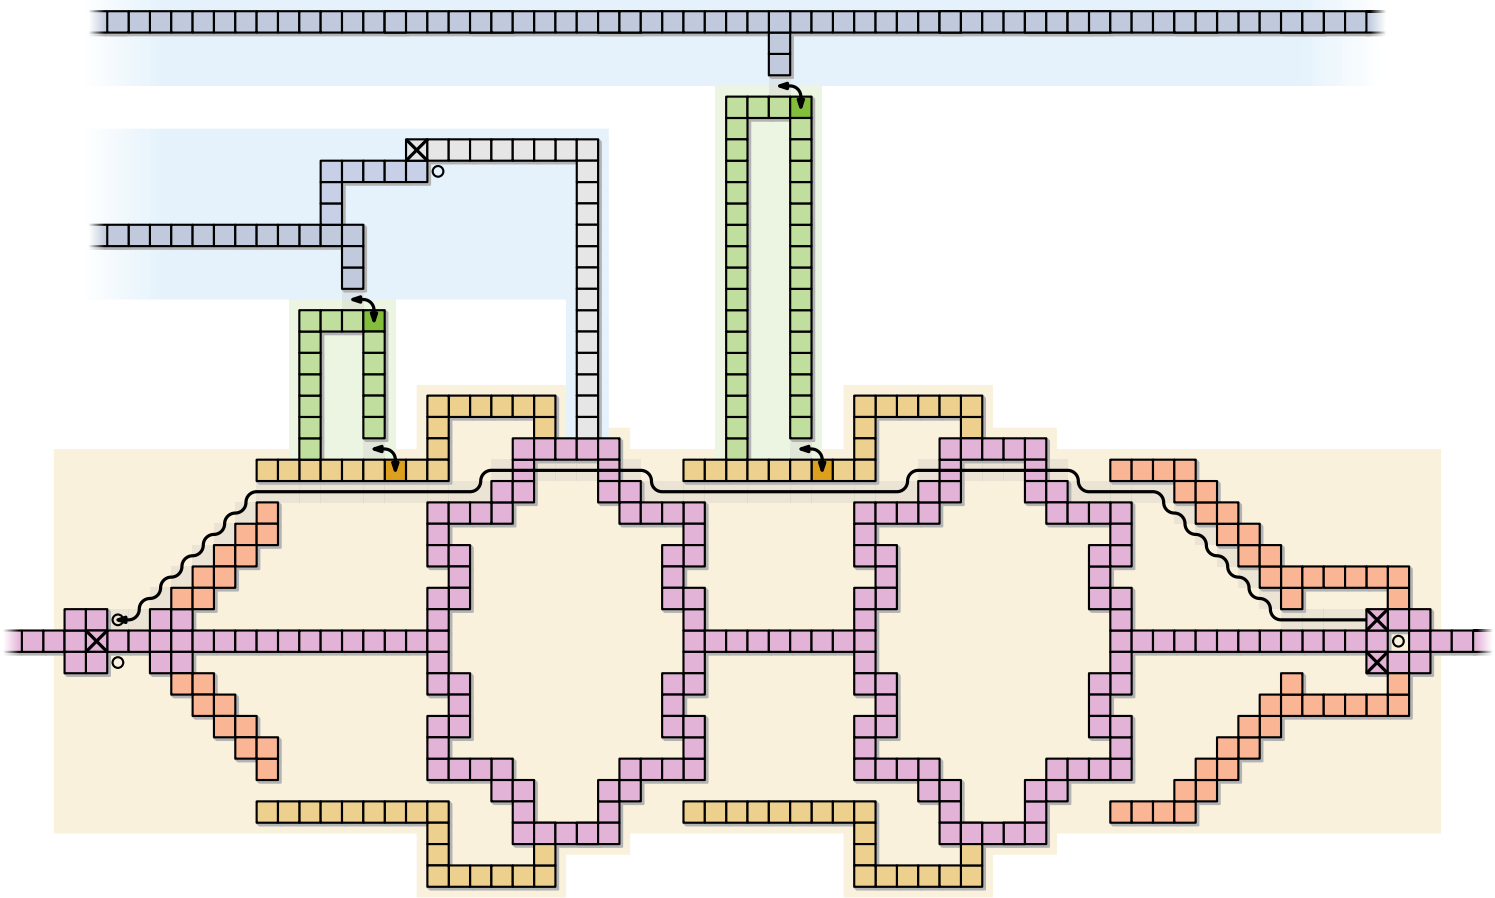

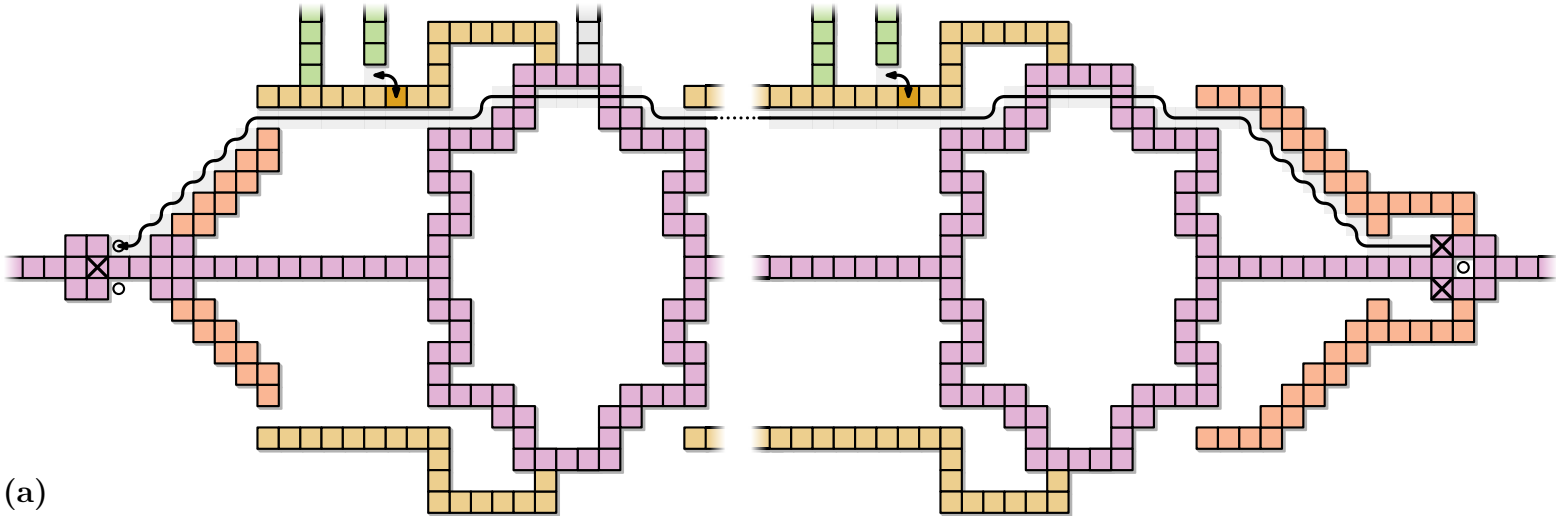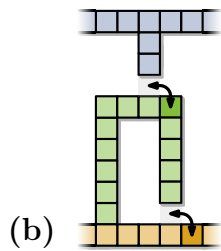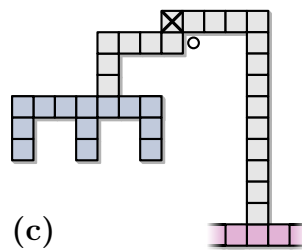

(a)

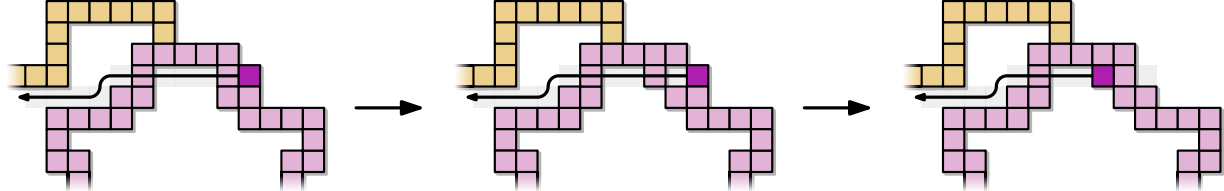

(b)

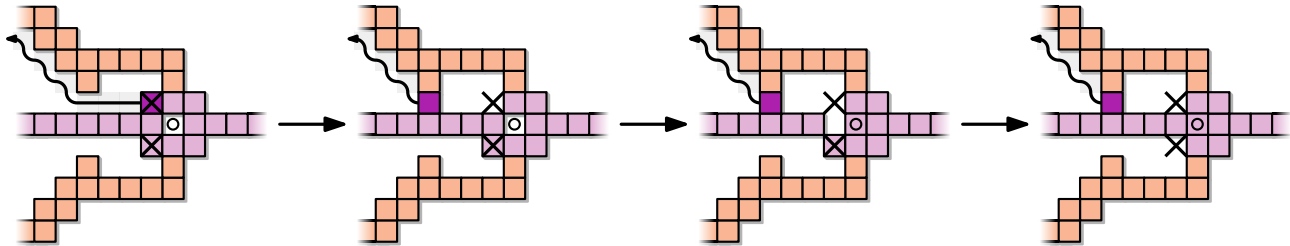

Supplement: Supplementary file 1 [file NPhard-gadgets-appendix.pdf]
